# Supplementary material for: Incremental Skill Learning of Stable Dynamical Systems
Source: arXiv:2003.11803 source file (2020-03-26)
Supplement: Supplementary file 1 [file AppendixLyapunov.tex]

\section*{Appendix: Lyapunov Theory} \label{Lyapunov_theorem}
In this section we recall some useful results concerning the stability of the equilibrium points of non-linear dynamical system. The reader is referred to \cite{Slotine91} for an exhaustive treatment of non-linear systems dynamics. 
 First, we recall the so-called \textit{Lyapunov theorem}  \cite{Slotine91}. The GAS of an equilibrium $\hat{\bfp}$ can be proved if a scalar function of the state variables $V_{f}(\bfp)$ satisfies:
\begin{subequations}
	\begin{align}
		&V_{f}(\bfp) > 0, ~\forall \bfp \neq \hat{\bfp} \label{eq:lyap_stab_cond1}\\
		&V_{f}(\bfp) = 0 \Longleftrightarrow \bfp = \hat{\bfp} \label{eq:lyap_stab_cond2}\\
		&V_{f}(\bfp) \rightarrow \infty ~\text{as}~ \Vert \bfp \Vert  \rightarrow \infty ~\text{(radially unbounded)} \label{eq:lyap_stab_cond3}\\
		&\dot{V}_{f}(\bfp) < 0, ~\forall \bfp \neq \hat{\bfp} \label{eq:lyap_stab_cond4}\\
		&\dot{V}_{f}(\bfp) = 0 \Longleftrightarrow \bfp = \hat{\bfp} \label{eq:lyap_stab_cond5}
	\end{align}	
	\end{subequations} 
A function that satisfies properties I-V is called a Lyapunov function. Moreover,
